# Supplementary material for: Deep Learning Segmentation of Complex Features in Atomic-Resolution Phase Contrast Transmission Electron Microscopy Images
Source: arXiv:2012.05322 source file (2020-12-09)

# DL+HRTEM Supplemental Information

The following graphs show the results of the hyperparameter grid search described in the paper. D refers to the depth of the network aka number of down convolution blocks in the network's contracting path, W refers to the number of features in the first block (W=4 means  $2^4$  features), and LR refers to the learning rate. We exhaustively tested through these hyperparameters to optimize the network and then selected the network with the best performance (D=4, W=5, LR=.0001).

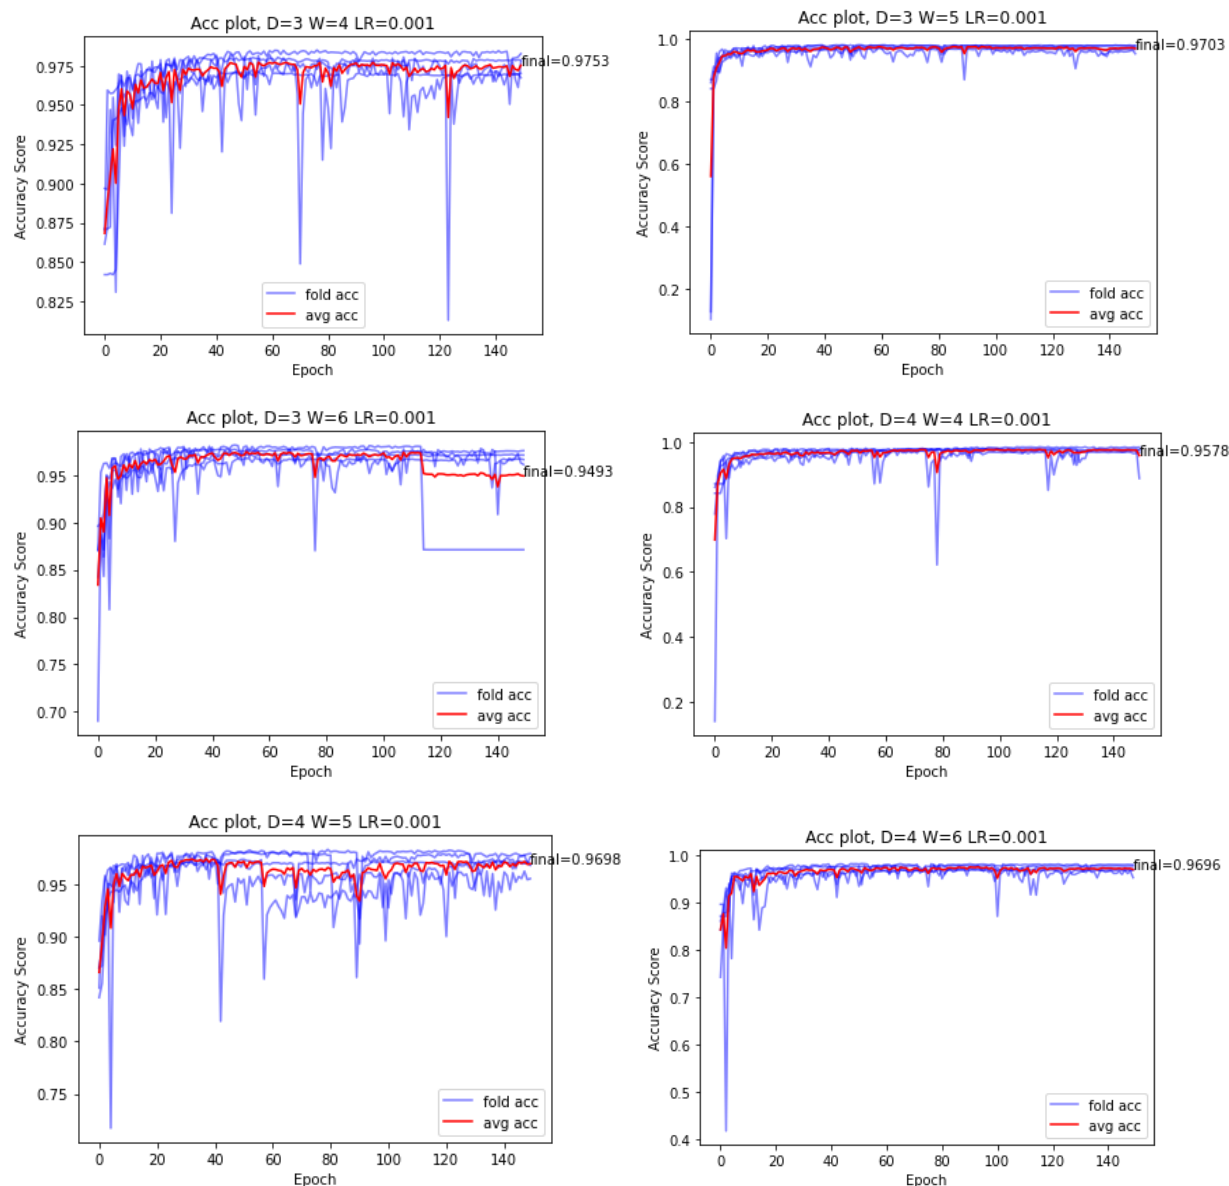

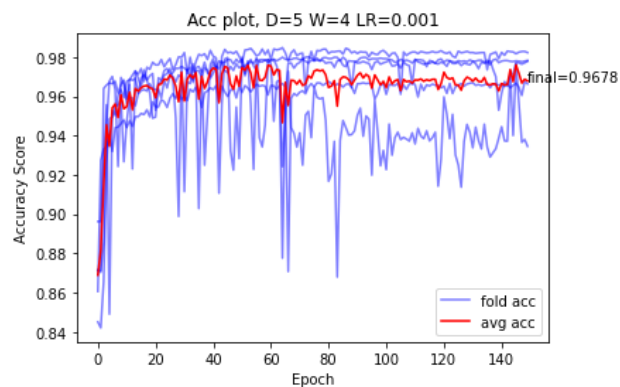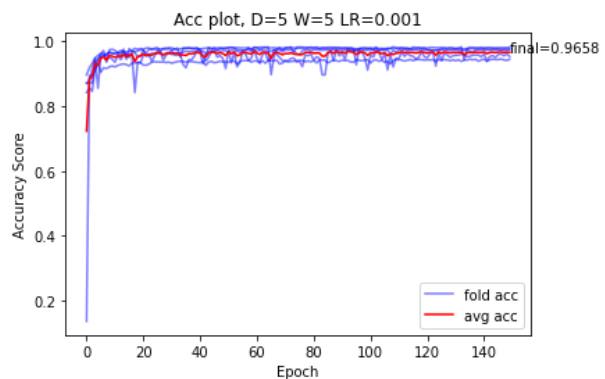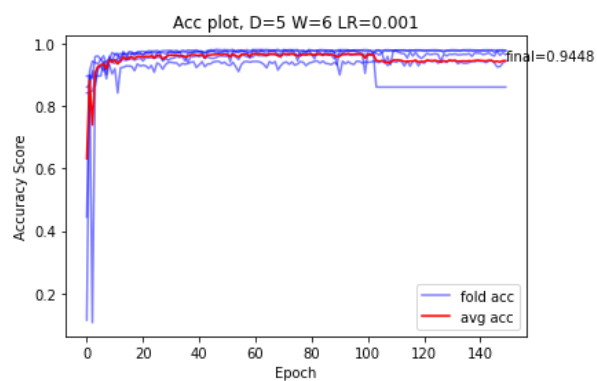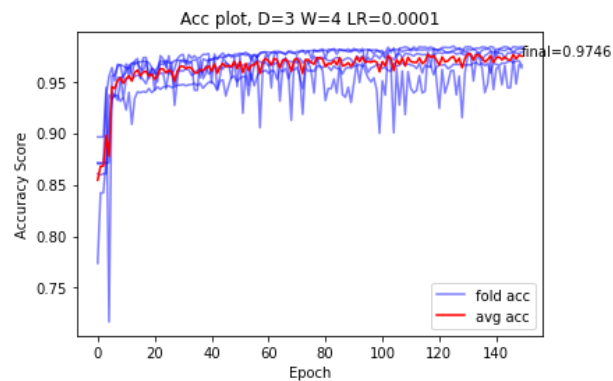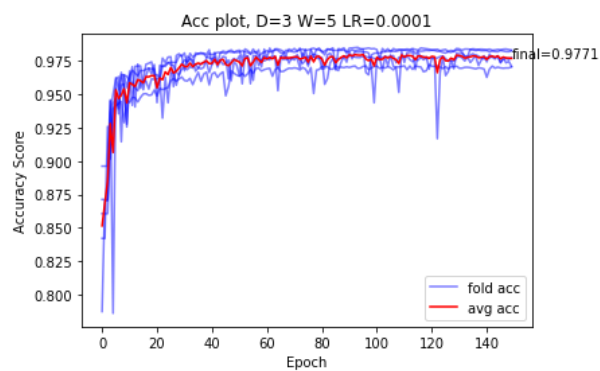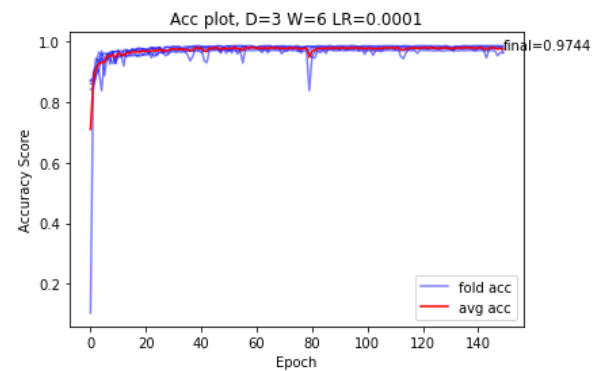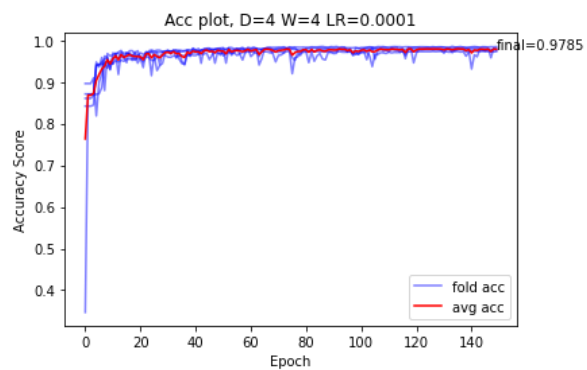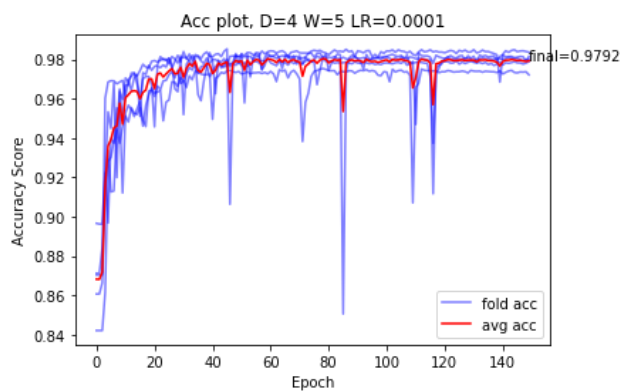

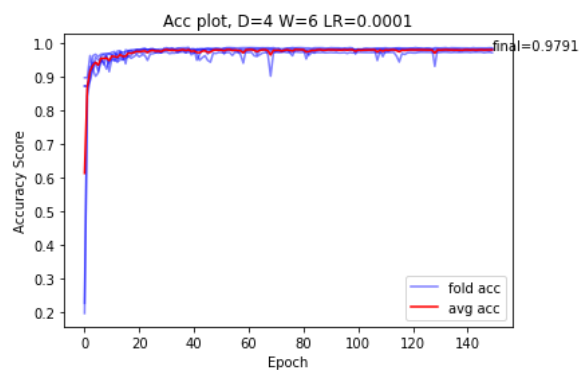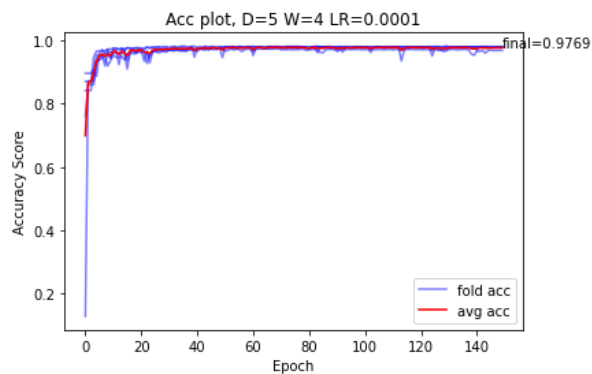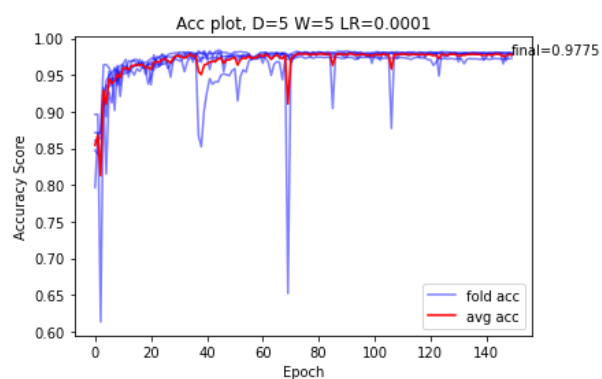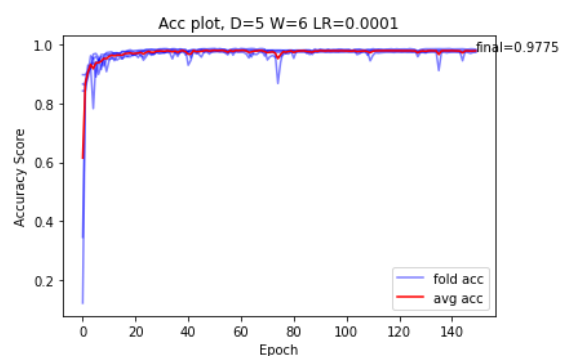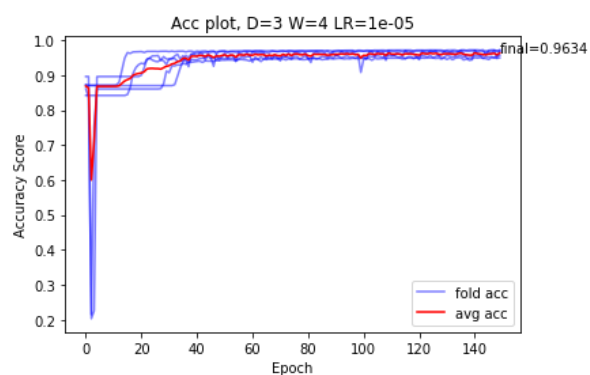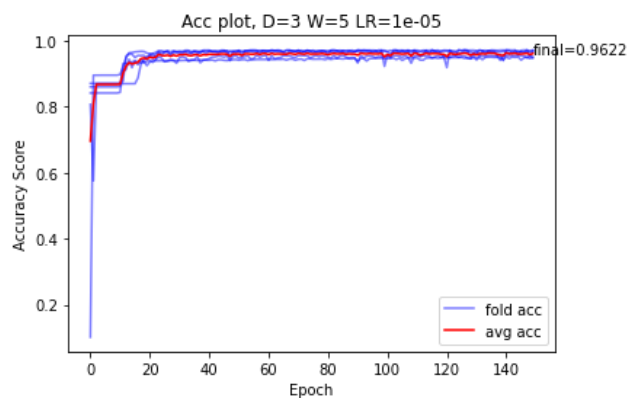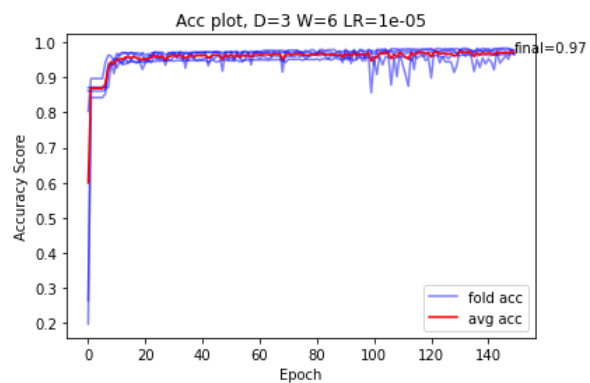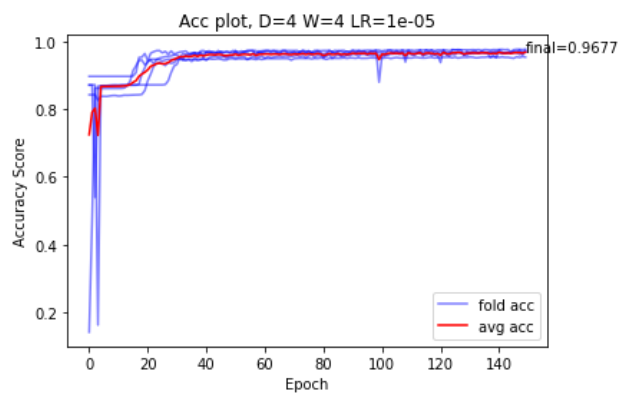

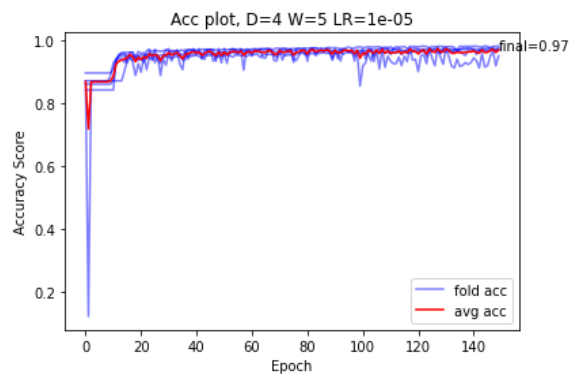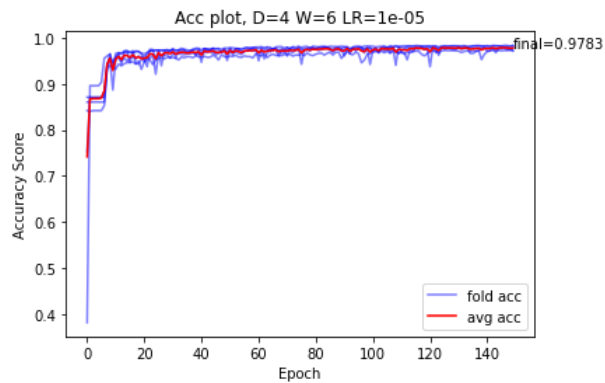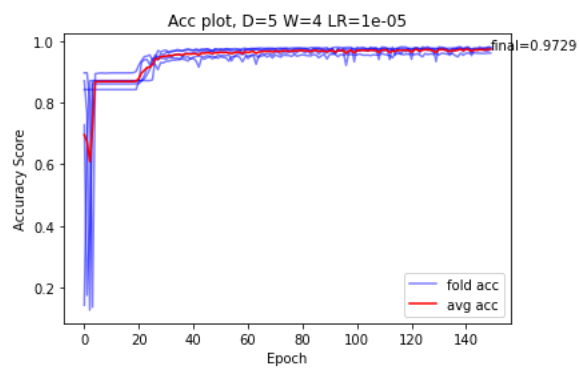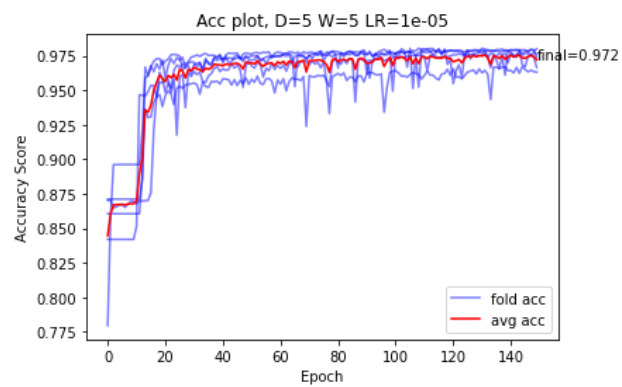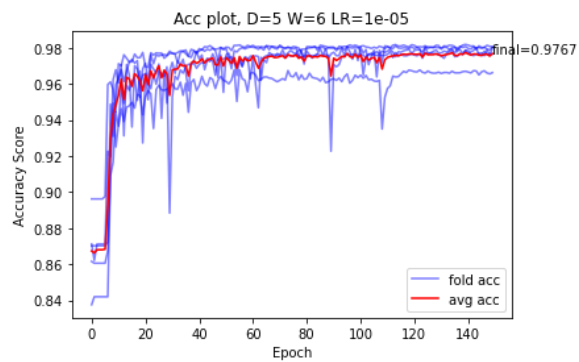

Supplement: Supplementary file 1 [file DL_HRTEM_Supplemental_Information.pdf]
